# Supplementary material for: Cost-Benefit Analysis of the Large Hadron Collider to 2025 and beyond
Source: arXiv:1507.05638 source file (2015-07-20)
Supplement: Supplementary file 1 [file supptable.pdf]

LHC-related costs covered by CERN by Programme and Subprogrammes and apportionment share to LHC (1993-2013; kEUR at 2013 constant prices)

| | Apportionmet share | LHC-related non-recurrent expense | LHC-related recurrent expense | LHC-related total cost |
|---|---|---|---|---|
| **Accelerators** | | **4,486,682** | **1,690,053** | **6,176,736** |
| CLIC | 0% | 0 | 0 | 0 |
| CNGS | 0% | 0 | 0 | 0 |
| Consolidation | 100% | 146,370 | 630 | 146,999 |
| Experimental Areas PS | 0% | 0 | 0 | 0 |
| Experimental Areas SPS | 0% (Codes EP, EPL, EPP) and 50% (Codes ASE, ATB, ESF, ESI) | 2,664 | 50,911 | 53,575 |
| General R&D | 0% <2007; 50% from 2008 | 1,760 | 727 | 2,487 |
| General Services | 0% <2007; 50% from 2008 | 1,480 | 11,052 | 12,533 |
| LEP | 0% | 0 | 0 | 0 |
| LHC | 100% | 4,076,429 | 1,111,295 | 5,187,724 |
| LHC injectors | 100% | 28,420 | 3,221 | 31,641 |
| LHC injectors upgrade | 100% | 14,103 | 186 | 14,289 |
| LHC upgrade | 100% | 153,252 | 3,218 | 156,470 |
| Low and medium energy | 0% | 0 | 0 | 0 |
| Medical applications | 0% | 0 | 0 | 0 |
| PS complex | 50% | 25,242 | 231,207 | 256,449 |
| R&D | 50% | 2,944 | 2,797 | 5,741 |
| R&D CLIC | 0% | 0 | 0 | 0 |
| SPS complex | 50% (Codes FSP, RFT) and 80% (Codes ASM, FAS, RFS, TSP) | 34,020 | 274,809 | 308,829 |
| **Administration** | | **9,325** | **314,484** | **323,809** |
| Administrative computing | 25% | 1,855 | 36,585 | 38,440 |
| Directorate | 25% | 3,438 | 84,329 | 87,767 |
| Finances | 25% | 716 | 30,729 | 31,444 |
| General Services | 25% | 1,400 | 24,705 | 26,105 |
| HR | 25% | 1,801 | 113,267 | 115,068 |
| Procurement | 25% | 115 | 24,869 | 24,984 |
| **Central expenses** | | **268** | **91,559** | **91,827** |
| bank charges and interests | 0% | 0 | 0 | 0 |
| Centralised personnel expenses | 25% | 0 | 56,968 | 56,968 |
| Housing fund | 0% | 0 | 0 | 0 |
| Insurances | 25% | 0 | 14,111 | 14,111 |
| Internal taxation | 0% | 0 | 0 | 0 |
| phone and postal charges | 25% | 0 | 1,101 | 1,101 |
| Storage management | 25% | 268 | 19,379 | 19,647 |
| **Infrastructure** | | **181,721** | **1,092,689** | **1,274,410** |
| Building construction | 80% | 69,728 | 0 | 69,728 |
| Computing | 20% | 5,124 | 27,702 | 32,826 |
| Energy | 20%<2000, then 50%, 80% as of 2008 | 155 | 478,824 | 478,979 |
| General Services | 50% | 0 | 438 | 438 |
| Medical service | 20%<2000, then 50%, 80% as of 2008 | 6,497 | 108,786 | 115,284 |
| Site facility | 40% | 83,850 | 468,111 | 551,961 |
| Technical infrastructure | 40% | 10,144 | 0 | 10,144 |
| Waste management | 40% | 6,223 | 8,828 | 15,050 |
| **Outreach** | | **20,053** | **141,812** | **161,865** |
| Communication | 80% | 15,274 | 104,498 | 119,772 |
| Exchange programmes | 50% | 0 | 19,008 | 19,008 |

| | | | | |
|---|---|---|---|---|
| Exchanges | 0% | 0 | 0 | 0 |
| Knowledge and Technology Transfer | 50% | 4,779 | 18,306 | 23,085 |
| Schools | 0% | 0 | 0 | 0 |
| **Pension Fund** | | **0** | **0** | **0** |
| Pension fund | 0% | 0 | 0 | 0 |
| **Research** | | **618,001** | **2,533,356** | **3,151,357** |
| Computing | 50% (Codes RSC, RSI) and 80% (Codes RCE, RCG, RCI, RCL) | 23,854 | 233,805 | 257,658 |
| Controls | 80% | 26 | 3,359 | 3,385 |
| Data analysis | 0% (Code RCX), 50% (Code RRD), 80% (Codes RDD, RDH) and 100% (Code RDA) | 8,959 | 71,736 | 80,695 |
| Electronics | 50% | 5,498 | 142,604 | 148,102 |
| EU supported R&D general | 50% | 25,572 | 1,192 | 26,763 |
| General Services | 50% | 26,345 | 291,565 | 317,910 |
| Grid computing | 80% | 1,447 | 2,813 | 4,260 |
| LHC computing | 100% | 126,539 | 161,380 | 287,919 |
| LHC detectors | 100% | 317,039 | 1,252,968 | 1,570,007 |
| LHC detectors upgrade | 100% | 78,328 | 272,638 | 350,966 |
| non-LHC physics | 0% | 0 | 0 | 0 |
| Theoretical physics | 50% | 4,394 | 99,297 | 103,691 |
| **Services** | | **3,039** | **17,441** | **20,480** |
| Electronics | 80% | 3,039 | 17,441 | 20,480 |
| **Total** | | **5,319,088** | **5,881,396** | **11,200,484** |
